# Supplementary material for: Strongly subradiant states in planar atomic arrays
Source: arXiv:2310.06791 source file (2023-10-10)

| Geometry of the structure                               |                                  | Square array/<br>square lattice                                                   |  | Square array/<br>centered-square<br>lattice                                        | Triangle array/<br>hexagonal lattice                                                | Hexagonal array/<br>hexagonal lattice                                               |                                                                                     |                                                                                     |
|---------------------------------------------------------|----------------------------------|-----------------------------------------------------------------------------------|--|------------------------------------------------------------------------------------|-------------------------------------------------------------------------------------|-------------------------------------------------------------------------------------|-------------------------------------------------------------------------------------|-------------------------------------------------------------------------------------|
|                                                         |                                  | 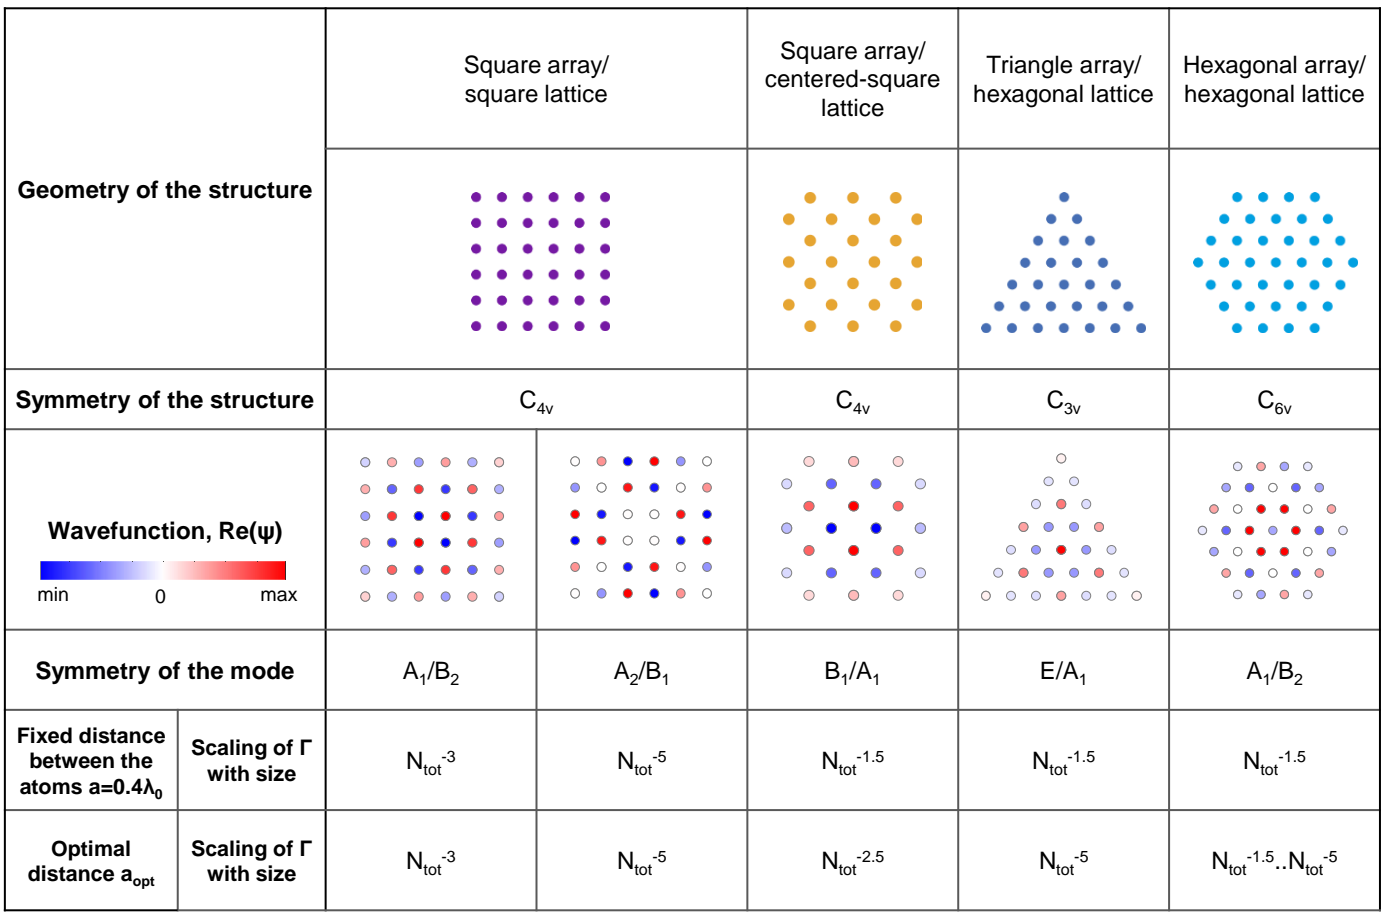 |  | 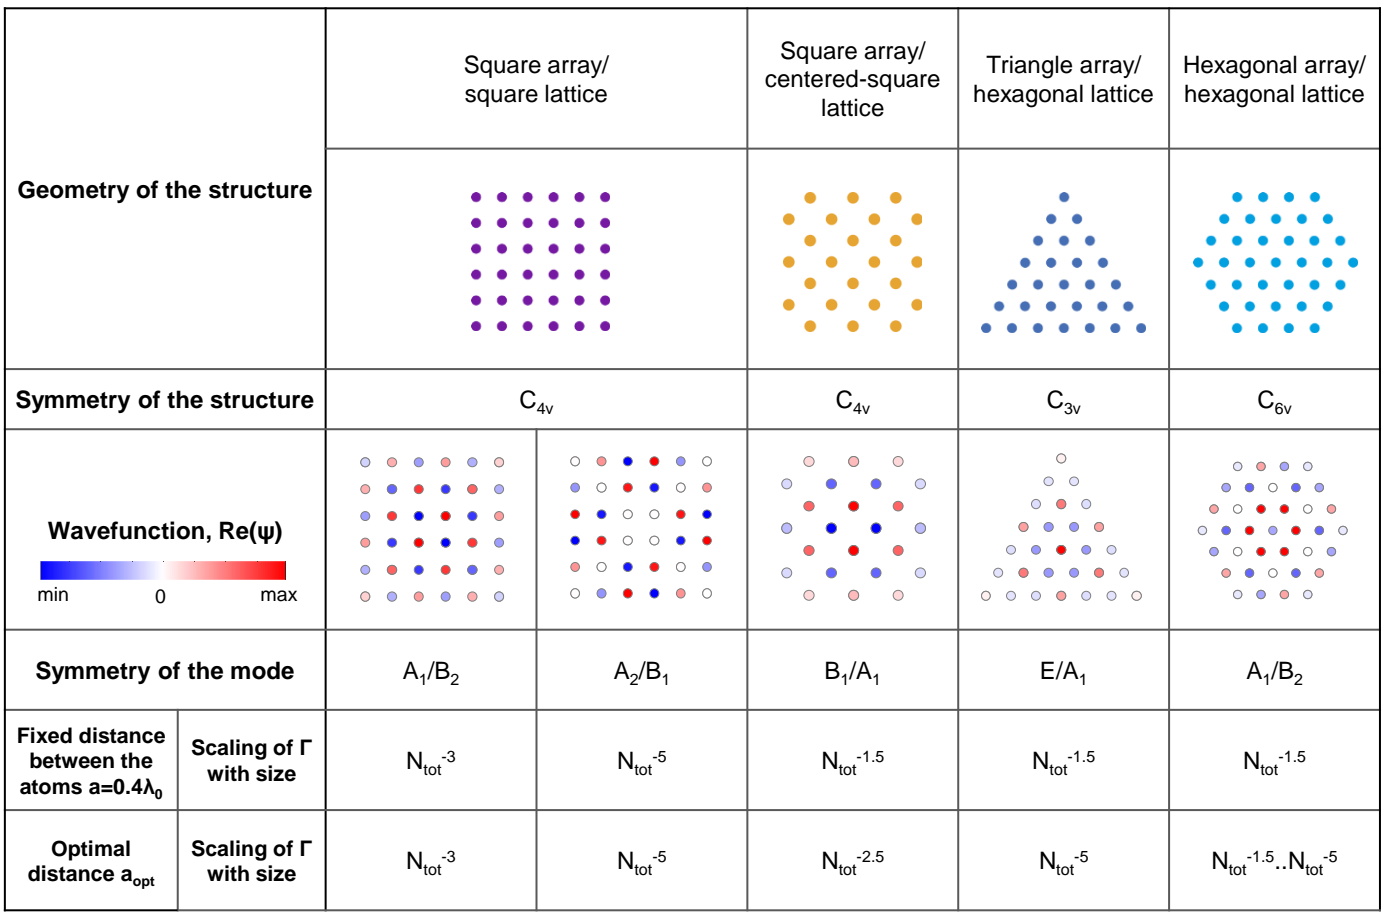 | 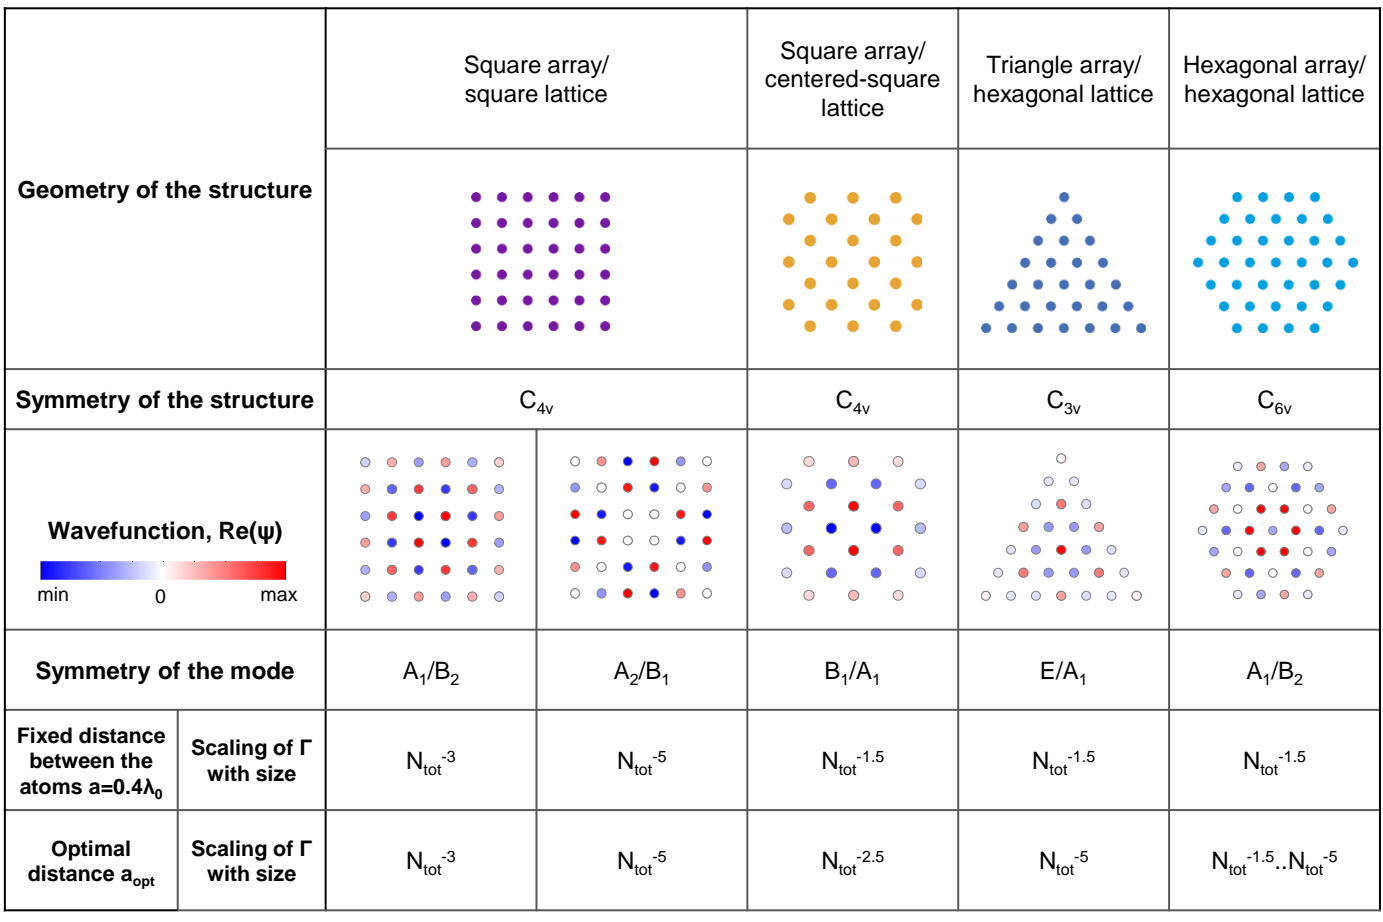 | 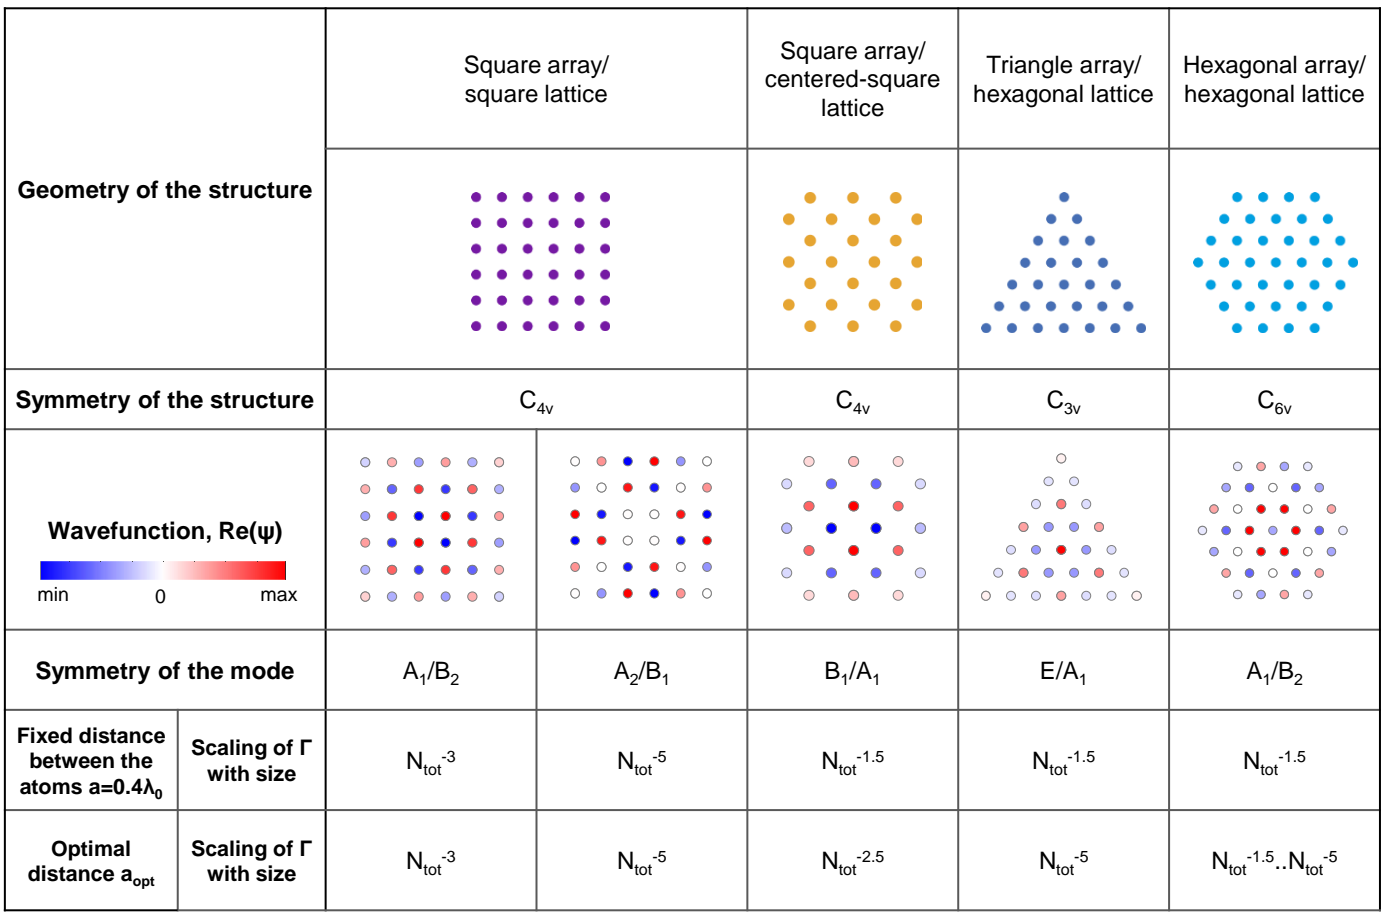 |                                                                                     |                                                                                     |
| Symmetry of the structure                               |                                  | $C_{4v}$                                                                          |  | $C_{4v}$                                                                           | $C_{3v}$                                                                            | $C_{6v}$                                                                            |                                                                                     |                                                                                     |
| Wavefunction, $\text{Re}(\psi)$                         |                                  | 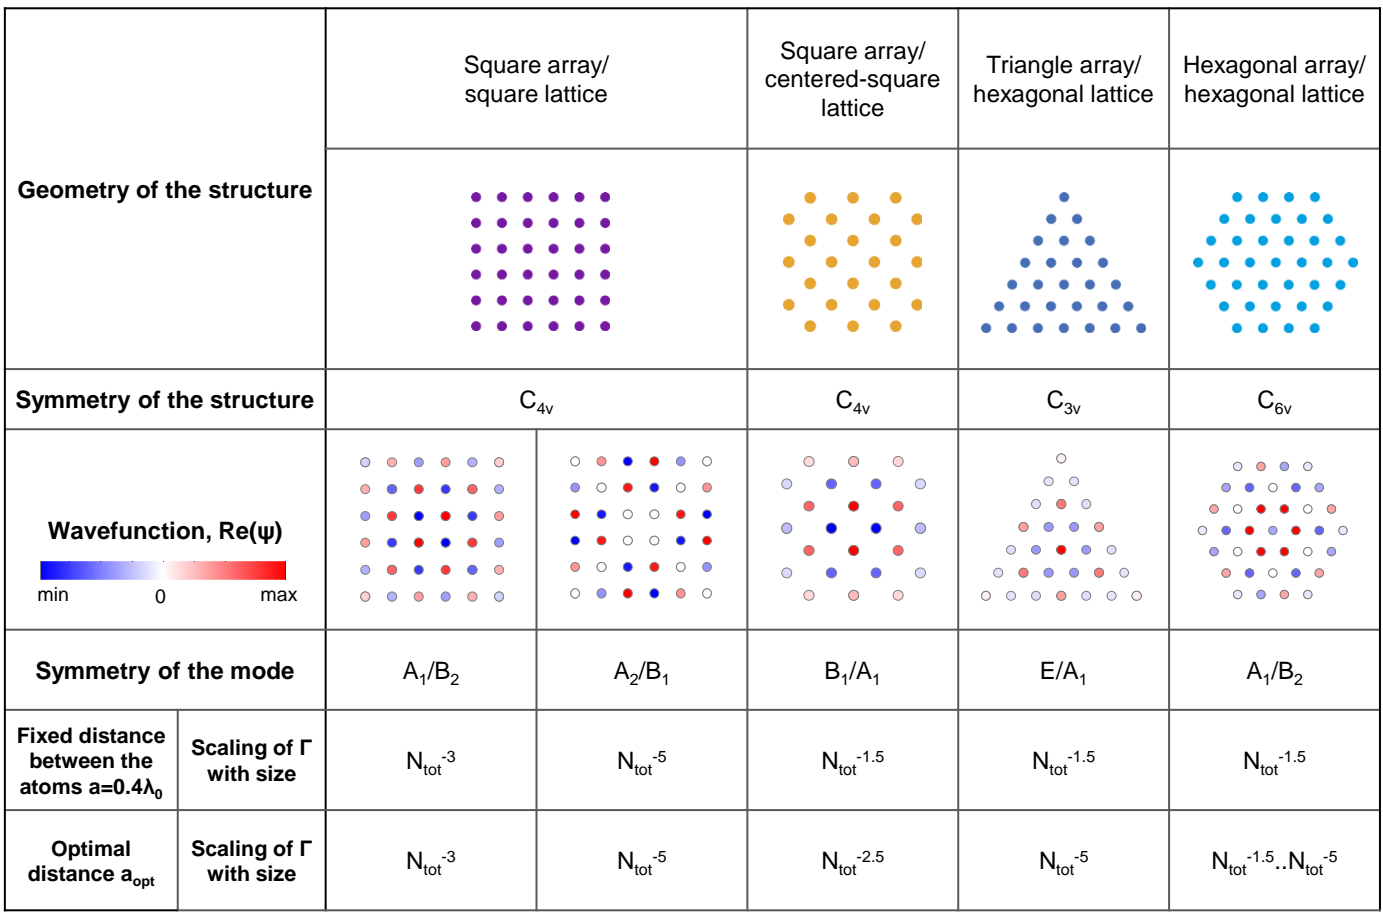  |  | 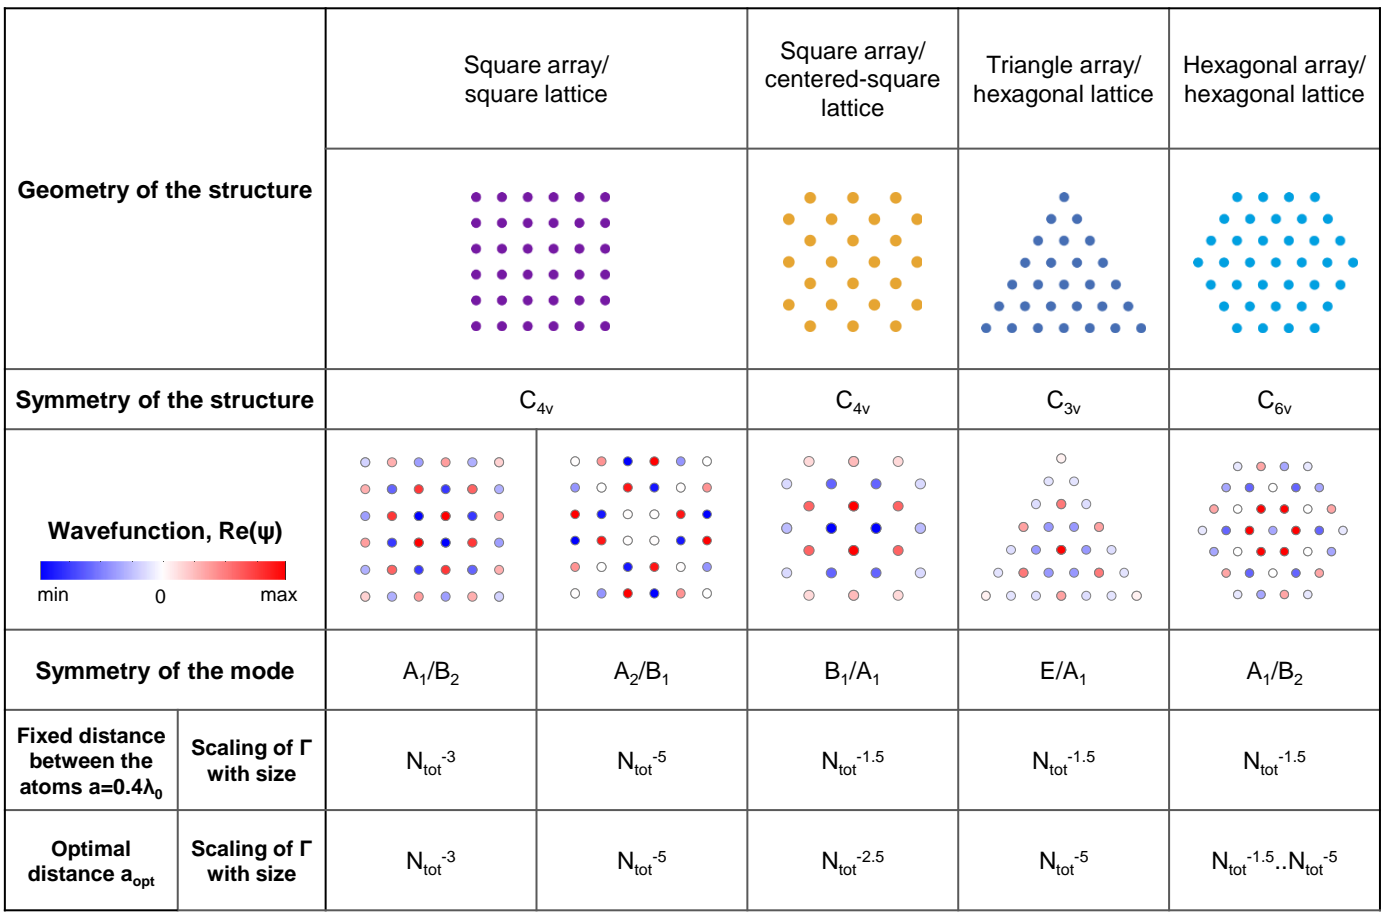  | 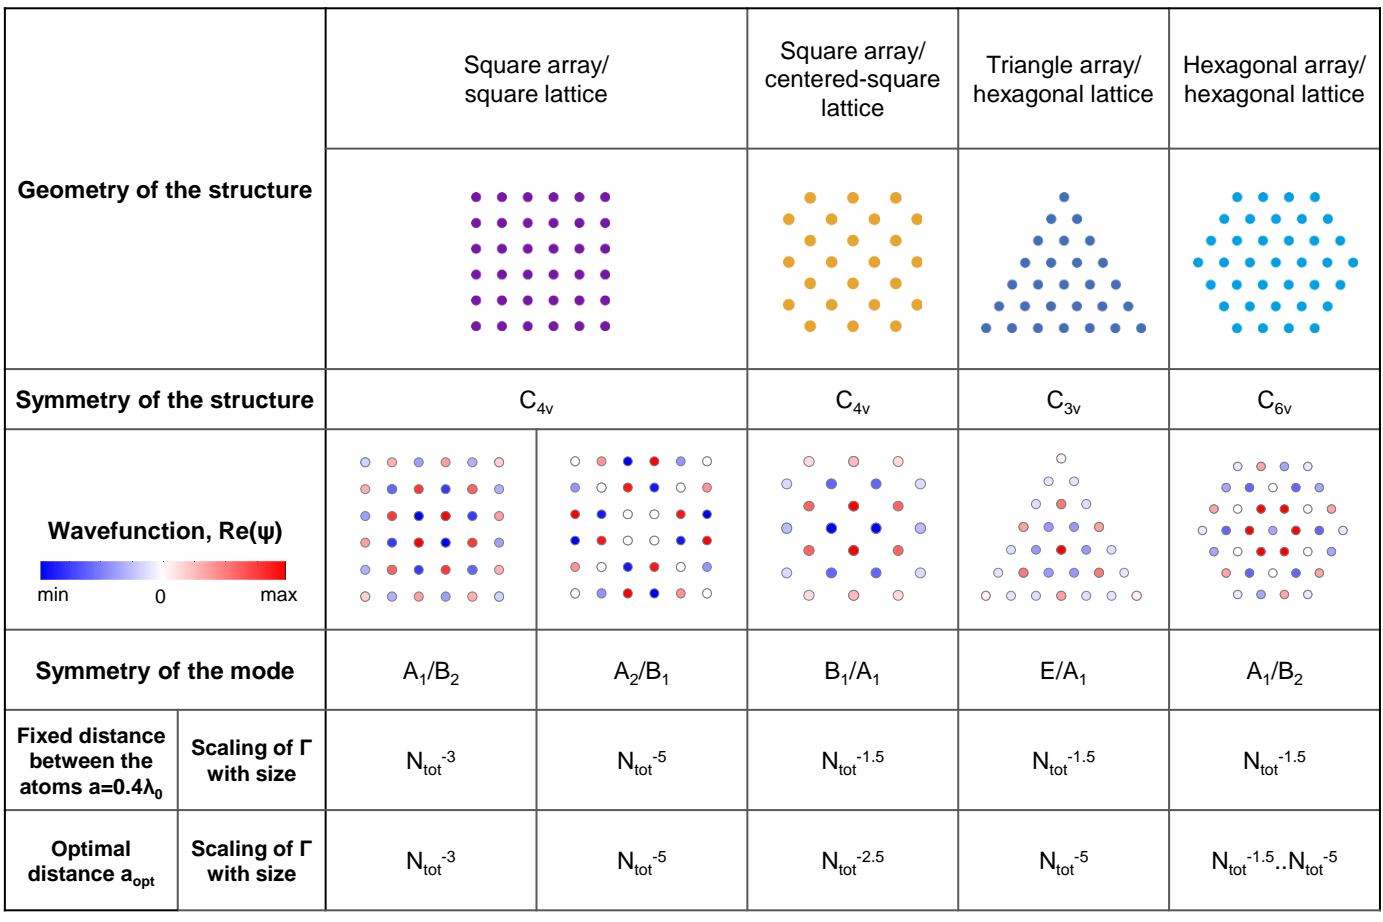   | 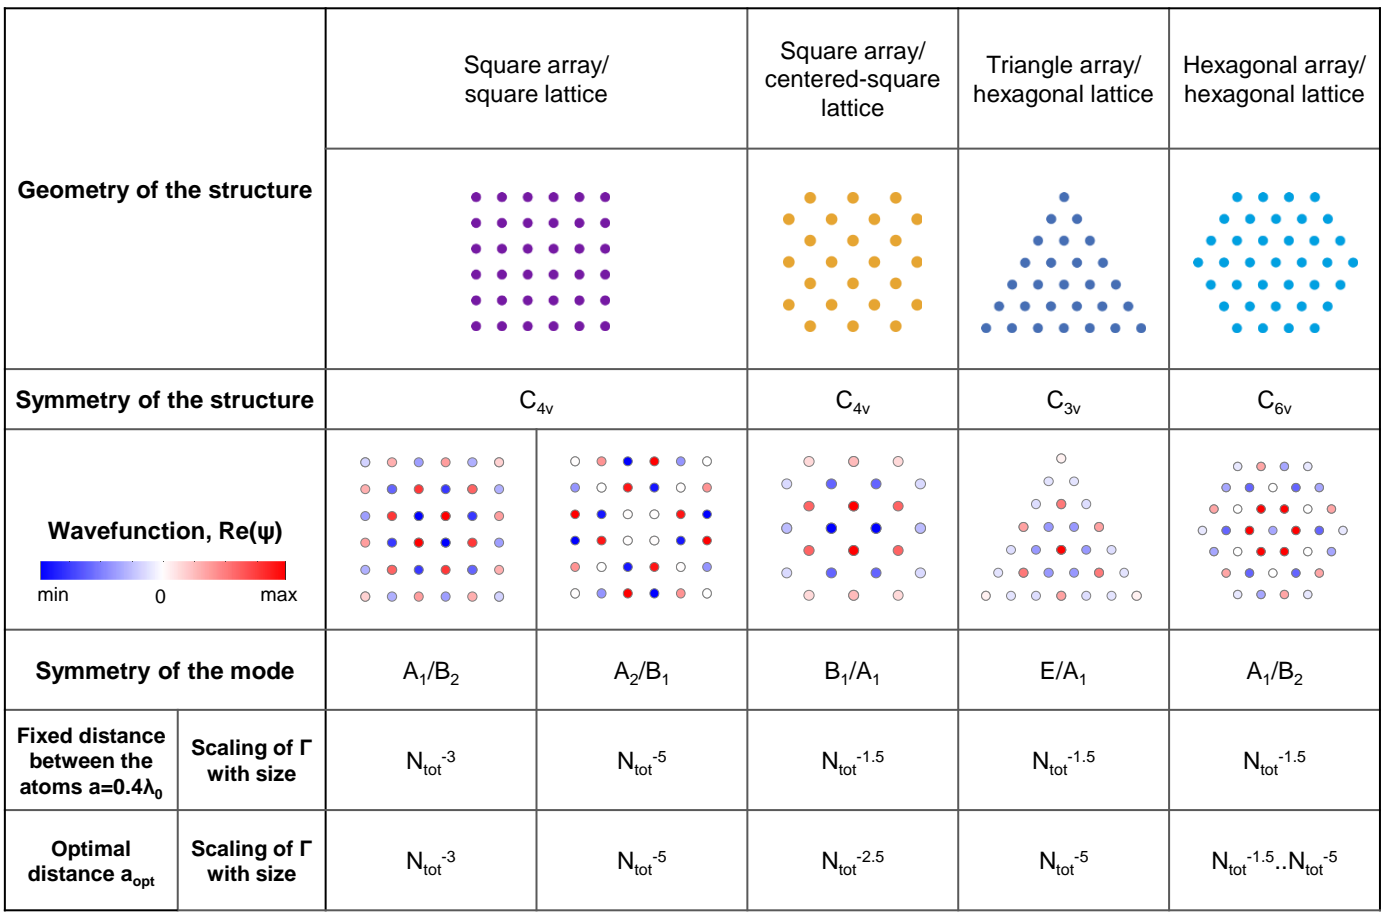  | 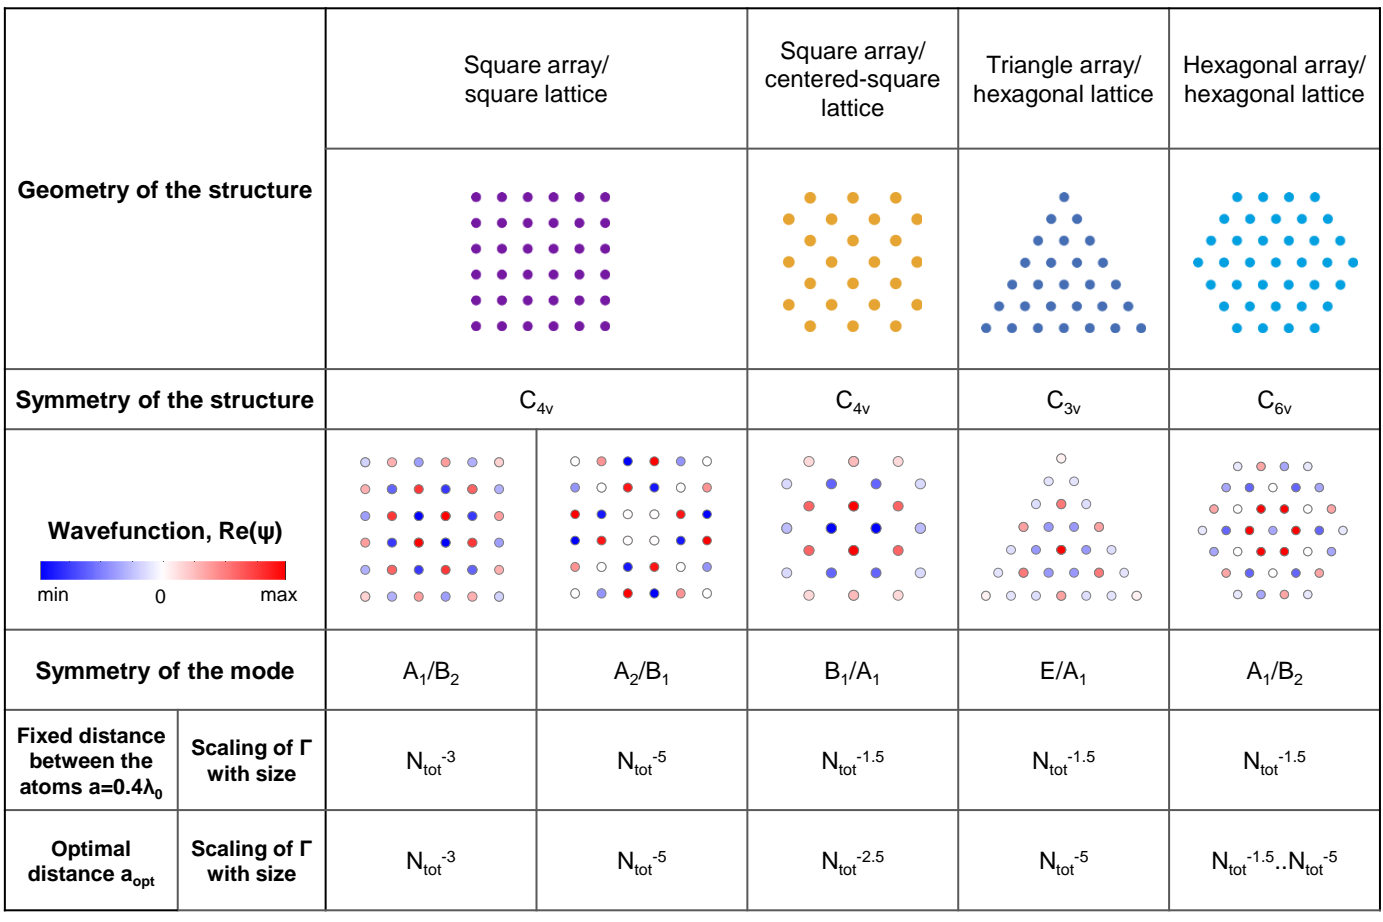 | 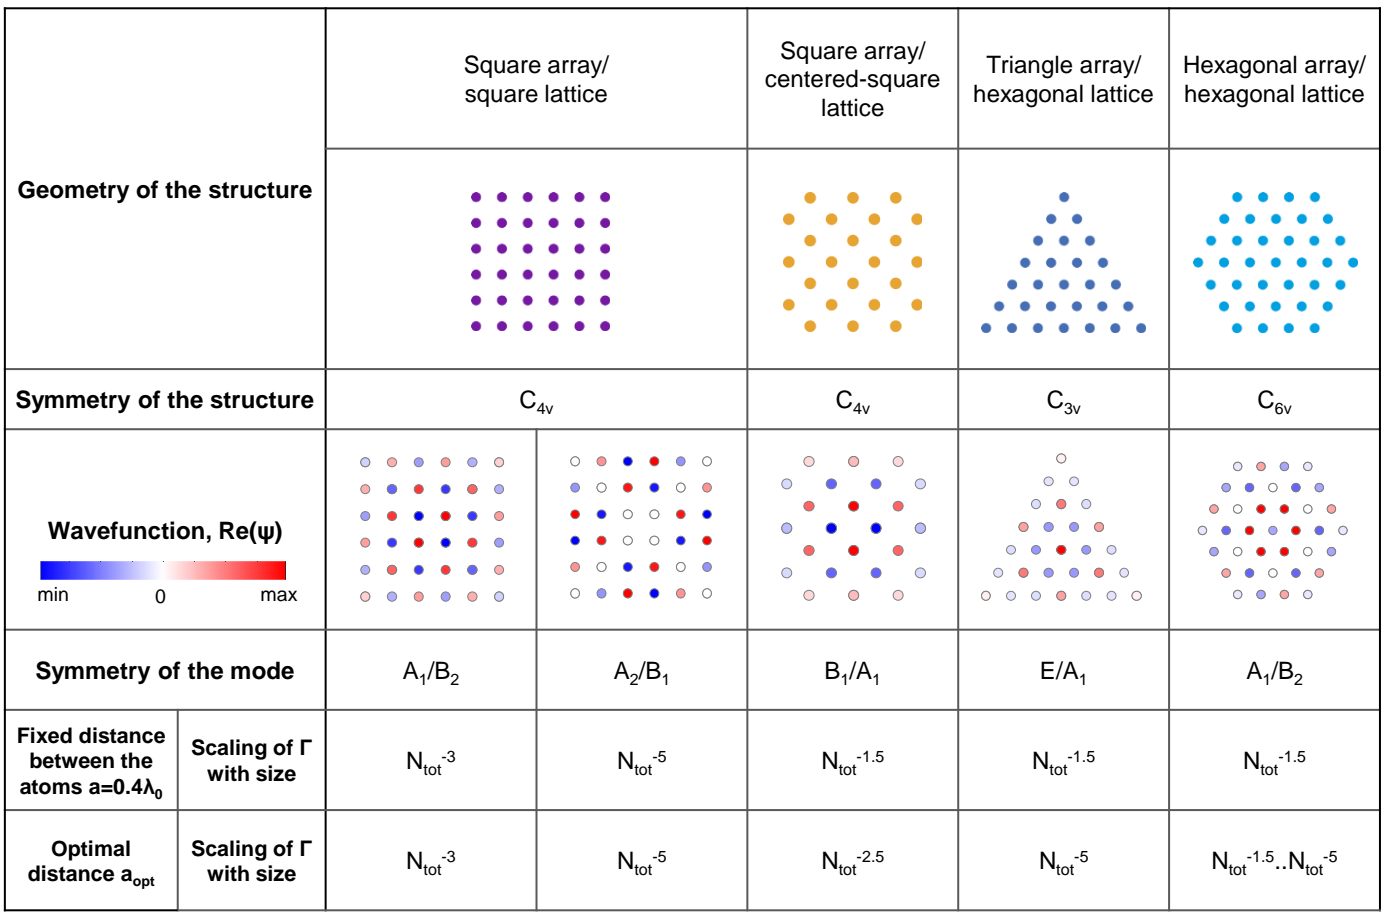 |
| Symmetry of the mode                                    |                                  | $A_1/B_2$                                                                         |  | $A_2/B_1$                                                                          | $B_1/A_1$                                                                           | $E/A_1$                                                                             | $A_1/B_2$                                                                           |                                                                                     |
| Fixed distance<br>between the<br>atoms $a=0.4\lambda_0$ | Scaling of $\Gamma$<br>with size | $N_{\text{tot}}^{-3}$                                                             |  | $N_{\text{tot}}^{-5}$                                                              | $N_{\text{tot}}^{-1.5}$                                                             | $N_{\text{tot}}^{-1.5}$                                                             | $N_{\text{tot}}^{-1.5}$                                                             |                                                                                     |
| Optimal<br>distance $a_{\text{opt}}$                    | Scaling of $\Gamma$<br>with size | $N_{\text{tot}}^{-3}$                                                             |  | $N_{\text{tot}}^{-5}$                                                              | $N_{\text{tot}}^{-2.5}$                                                             | $N_{\text{tot}}^{-5}$                                                               | $N_{\text{tot}}^{-1.5}..N_{\text{tot}}^{-5}$                                        |                                                                                     |

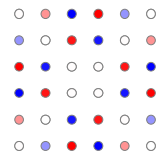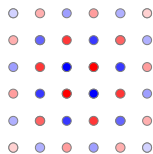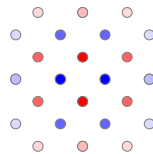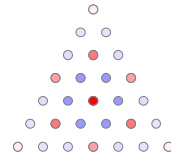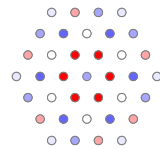

Supplement: Supplementary file 1 [file Table_different_geometries_v3.pdf]
